# Supplementary material for: Dia- and adiabatic dynamics in a phononic network
Source: arXiv:2011.08080 ancillary file (2020-11-16)
Supplement: Supplementary file 1 [file SI.pdf]

# Supplemental Material: Dia- and adiabatic dynamics in a phononic network

Daniel Schwienbacher,[1,2,3,*] Thomas Luschmann,[1,2,3,†] Rudolf Gross,[1,2,3] and Hans Huebl[1,2,3,‡]

[1] *Walther-Meißner-Institut, Bayerische Akademie der Wissenschaften, Walther-Meißner-Str. 8, 85748 Garching, Germany*

[2] *Physik Department, Technische Universität München, James-Franck-Str. 1, 85748 Garching, Germany*

[3] *Munich Center for Quantum Science and Technology (MCQST), Schellingstr. 4, 80799 München, Germany*

(Dated: November 14, 2020)

* These two authors contributed equally; daniel.schwienbacher@wmi.badw.de

† These two authors contributed equally

‡ hans.huebl@wmi.badw.de

### A. Coupling between two resonant modes

To extract the intrinsic coupling strength of two modes $\alpha$ amd $\beta$ we tune the system in such a way, that the independent crossing approximation (ICA) [S1] can be applied. This approximation, introduced by Brundobler et al. [S1], states that between coupled modes energy transfer only occurs if the mode frequencies $\Omega_\alpha$ and $\Omega_\beta$ differ not much stronger than their coupling rate $g_{\alpha\beta}$. Thus, a pair of modes far detuned from all other modes can be treated as independent. In our system we can obtain this for example by detuning the third mode far from the coupled modes. In this case the standard Landau-Zener case of two crossing modes can be applied [S2–S4], described by the Hamiltonian:

$$H^{(2)} = \hbar \begin{pmatrix} \Omega_\alpha & g_{\alpha\beta} \\ g_{\alpha\beta} & \Omega_\beta \end{pmatrix} \tag{S1}$$

Here $\Omega_\alpha$ and $\Omega_\beta$ are the undisturbed, resonance frequencies of the modes $\alpha$ and $\beta$ which can be tuned tuned, and $g_{\alpha\beta}$ is the mutual coupling rate between them. The eigenvalues of Eq. S1 are [S5]:

$$\Omega_\pm^{\alpha,\beta} = \frac{1}{2}\left[\Omega_\alpha + \Omega_\beta \pm \sqrt{\left(\Omega_\alpha - \Omega_\beta\right)^2 + 4g_{\alpha\beta}^2}\right] \tag{S2}$$

which describe the dressed states formed by the coupled modes. For large detuning of the mode frequencies $|\Omega_\alpha - \Omega_\beta| \gg g_{\alpha\beta}$ the frequencies are those of the undisturbed modes. In the case of zero detuning $\Omega_\alpha - \Omega_\beta = 0$, the modes interact and the characteristic frequency splitting difference between the two dressed states is given by: $\Omega_+^{\alpha,\beta} - \Omega_-^{\alpha,\beta} = \sqrt{4g_{\alpha\beta}^2} = 2g_{\alpha\beta}$. This enables the extraction of the bare coupling strength from a measurement of an avoided crossing between two modes, if the third mode is far detuned. If the modes themselves are sufficiently far detuned $\Delta_{ij} = \Omega_i - \Omega_j$ from each other we can extract the undisturbed resonance frequency of the strings and relate them to their mechanical properties:

$$\Omega_i^n = \frac{n\pi}{l}\sqrt{\frac{\sigma_0}{\rho}}, \tag{S3}$$

with the mode number $n$ the string length $l$, pre-stress $\sigma_0$ and density $\rho$. Here, $i$ indicates the specific mode $(\alpha, \beta, \gamma)$ of the system, corresponding to the string (A,B,C).

### B. Data acquisition techniques

To study the system we employ two different data acquisition techniques. To characterize the system with all the resonance frequencies and $Q$-factors, the coupling strengths between the strings as well as to show the full in-situ control over the string network, we use a frequency domain (FD) setup in which we use a vector network analyzer (VNA). Using a VNA, we send a drive tone to the piezo-actuator and compare it to the measured driven mechanical response of a string, encoded in the voltage signal of a photo-detector. Alternatively we use a spectrum analyzer (SA) to measure the thermal motion spectrum of a string (Fig. S1).
To investigate the dynamics of the nano-string network we employ a time domain (TD) measurement setup. For this we use an arbitrary wave generator and a pulsed source to send excitation pulses to the system, and a digitizer card with up to $200 \cdot 10^6$ samples/s to acquire the photo-detector's AC signal and thereby measure the mechanical excitation of a selected string. A full measurement of the system in the TD case is achieved by repeating a measurement while consecutively changing the readout string (A,B,C) as shown in Fig. 4 in the main text.

### C. In-situ tuning mechanism

The in-situ frequency control scheme used, follows the one reported in Ref. [S6], we refer to there for the full description of the mechanism. By strongly driving a higher harmonic of a string using an auxiliary drive tone with frequency $\Omega_{\mathrm{aux}}$, this mode enters the non-linear Duffing regime [S7, S8]. In this case, the string experiences a finite elongation due to the large displacement. This elongation leads to an additional pre-stress $\Delta\sigma$ to the tensile pre-stress $\sigma_0$ in the material. The total stress $\sigma = \sigma_0 + \Delta\sigma(\Omega_{\mathrm{aux}}))$ then translates to a change in resonance frequency for all harmonics of the string. A classical Duffing oscillator exhibits a bi-stability within a certain frequency range if the system is driven above the critical amplitude [S7]. In this regime, high powers allow to change the pre-stress.

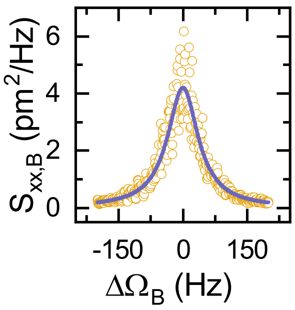


FIG. S1. Thermal displacement spectrum of string B, showing an intrinsic FHWM of $\Gamma_B = 86\,\text{Hz}$. Line is a Lorentzian fit to the data, used to extract the linewidth and frequency.

| | A | B | C |
|---|---|---|---|
| $\Omega^0/2\pi$ | 9.2382 MHz | 9.2463 MHz | 9.2538 MHz |
| $\Gamma/2\pi$ | 80(10) Hz | 80(10) Hz | 80(10) Hz |
| | | | |

TABLE I. Eigenfrequencies of the undisturbed modes of the string resonators (A,B,C) and their linewidth (FWHM). The values for the single strings were extracted from thermal displacement spectra of the respective strings. For string B such a spectrum can be seen in Fig. S1

Interestingly, the amplitude of the excited mode can also be tuned via the drive frequency $\Omega_{\text{aux}}$, as the amplitude follows the characteristic shark-fin shape of the amplitude of the oscillator. The extend of this frequency range limits the range in which the fundamental frequency of a string can be tuned. If the auxiliary tone used to drive the higher harmonic leaves this bi-stability region, the frequency shift imposed onto the fundamental mode vanishes. Due to the high amplitudes and thus also driving forces necessary to in-situ tune all three strings at the same time, the power dissipation in the piezo actuator can lead to an increase in the overall sample temperature over the course of a measurement. In our analysis we corrected for this linear effect.

### D. Characteristic sample parameters

To extract the undisturbed eigenfrequencies of the single strings, thermal displacement spectra of the respective strings were used. In Fig. S1 this is exemplarily shown for string B. By fitting the data in this thermal displacement spectrum with a Lorentzian line-shape, we extracted the intrinsic resonance frequency $\Omega^0_\beta$ and linewidth $\Gamma_\beta$ (FWHM). The values for all three strings are summarized in Tab. I  To extract the coupling strengths between each pair of strings, we used the independent crossing approximation. By tuning two modes into resonance with each other while keeping the third mode far detuned, we can treat the resulting avoided crossing as independent. The system can then be described by (S1) and the coupling strength can be extracted as discussed before. The coupling inter mode coupling strengths for the system are summarized in Tab. II.

| | $\alpha\beta$ | $\beta\gamma$ | $\alpha\gamma$ |
|---|---|---|---|
| $g_{ij}/2\pi$ | 640.5 Hz | 615 Hz | 653.5 Hz |

TABLE II. Experimentally determined inter-modal couplings

### E. Classical equation of motion for a coupled oscillator system

An alternative viewpoit to (S2) is to discuss the equation of motion of two coupled harmonic oscillators. We follow here the approach of Novotny [S5] and model the coupled systems by

$$\begin{aligned} -\kappa_{\alpha\alpha} x_\alpha + \kappa_{\alpha\beta}(x_\beta - x_\alpha) &= m_\alpha \ddot{x}_\alpha, \\ -\kappa_{\beta\beta} x_\beta + \kappa_{\beta\alpha}(x_\alpha - x_\beta) &= m_\beta \ddot{x}_\beta, \end{aligned} \tag{S4}$$

where we have introduced the effective spring constant of the strings $\kappa_{\alpha\alpha}$ and $\kappa_{\beta\beta}$, as well as the coupling mediated by the neighboring string in terms of the spring constants $\kappa_{\alpha\beta}$=$\kappa_{\beta\alpha}$. The mass of the mode, which equals the mass of the strings are $m_\alpha$ and $m_\beta$ and $x_\alpha$ and $x_\beta$ denote the displacements. When mode $\alpha$ and $\beta$ are resonant, the eigenfrequencies become modified and can be associated with dressed states. Here, the characteristic anticrossing is given by the frequency splitting, which we have identified with $2g_{\alpha\beta}$ in Sec. A. According to Ref. [S5],

$$g_{\alpha\beta} = \frac{1}{2} \frac{\sqrt{\kappa_{\alpha\beta}/m_\alpha}\sqrt{\kappa_{\alpha\beta}/m_\beta}}{\sqrt{\tilde{\Omega}_\alpha \tilde{\Omega}_\beta}} \tag{S5}$$

with $\tilde{\Omega}_\alpha = \sqrt{(\kappa_{\alpha\alpha} + \kappa_{\alpha\beta})/m_{\mathrm{A}}}$ and $\tilde{\Omega}_\beta = \sqrt{(\kappa_\beta \beta + \kappa_{\alpha\beta})/m_{\mathrm{B}}}$. For our system, we can well use the approximations $m_\alpha = m_\beta = m$, $\tilde{\Omega}_\alpha \approx \tilde{\Omega}_\beta$, and $\kappa_{\alpha\alpha} = \kappa_{\beta\beta}$. Then (S5) simplifies to

$$g_{\alpha\beta} \approx \frac{1}{2} \frac{\kappa_{\alpha\beta}}{m\tilde{\Omega}_\alpha}. \tag{S6}$$

This relation allows us to connect the experimentally determined coupling rate with the parameters used in the coupled equations of motion.

### F. Numerical simulation of the steady state observation and state transfer dynamics

To investigate the nature of the beating frequencies between the two hybridized modes in the diabatic limit of the state transfer measurement, we examplarily take one tuning speed $(\zeta_\alpha/2\pi)^{-1} = 25\,\mu\mathrm{s/kHz}$ and look at the experimentally determined and numerically calculated amplitudes of the strings B and C in this case. This is shown in Fig. S2. By using a Fourier transformation on the data, we can determine the frequency of the beating oscillation between the strings and find a frequency of $\nu_{\mathrm{R}} \approx 3270(320)\,\mathrm{Hz}$ which corresponds to the modesplitting between the $\beta$ and $\gamma$ mode. The extracted frequencies agree with the numerical simulation and the experiment within the confidence interval. Furthermore the extracted frequencies are also in agreement with the coupling strength between the two hybridized modes $g_{\beta\gamma}/2\pi = 615\,\mathrm{Hz}$ (cf. Table II). The dynamics of the system, in the general case, can not be described analytically [S1]. However, numeric simulations are still viable. For this, we consider the equations of motion for three coupled modes:

$$m_i \ddot{x}_i + m_i \Gamma_i \dot{x}_i + \kappa_{ii} x_i = \kappa_{ij}(x_j - x_i) + \kappa_{jk}(x_k - x_i) + F_{\mathrm{drive}} \tag{S7}$$

with $i, j, k \in \{\alpha, \beta, \gamma\}$. Here, $\Gamma_i$ denotes the individual damping rate of the string $i$, $\kappa_{ii}$ is the (effective) spring constant of the string. The spring constants $\kappa_{ij}$ and $\kappa_{ik}$ describe the force originating from the neighbouring strings. In addition, we consider the excitation force $F_{\mathrm{drive}}$. Under the approximation of nearly identical strings, we set $\Gamma_\alpha = \Gamma_\beta = \Gamma_\gamma \equiv \Gamma$ as well as $m_\alpha = m_\beta = m_\gamma \equiv m$. Without loosing generality, we can now focus on one string, which we excite at the beginning of the state transfer protocol. We choose string A for this purpose to be later able to compare the model with the experimental data. Therefore, $\Omega_\alpha$ is time dependent. In particular, to model our experiment we choose

$$\Omega_\alpha(t) = \begin{cases} \Omega_\alpha^0 & t < t_0 \\ \Omega_\alpha^0 + \zeta_\alpha(t - t_0) & t_0 \le t \le t_0 + \tau \\ \Omega_\alpha^0 + \Delta\Omega_\alpha & t \ge t_0 + \tau \end{cases} \tag{S8}$$

with $\zeta_\alpha = \Delta\Omega_\alpha/\tau$. We can now use this set of equations (S7) with the definition of $\Omega_\alpha(t)$ to either calculate the case of all three resonators matching in frequency using a steady-state perspective and thus reproduce the experimental situation of Fig. 3a). The result of this is depicted in Fig. 3c) in form of the squared displacement amplitude. In addition, we can simulate the coupled differential equations (S7) for each $\zeta_\alpha$ to model the experimental data depicted

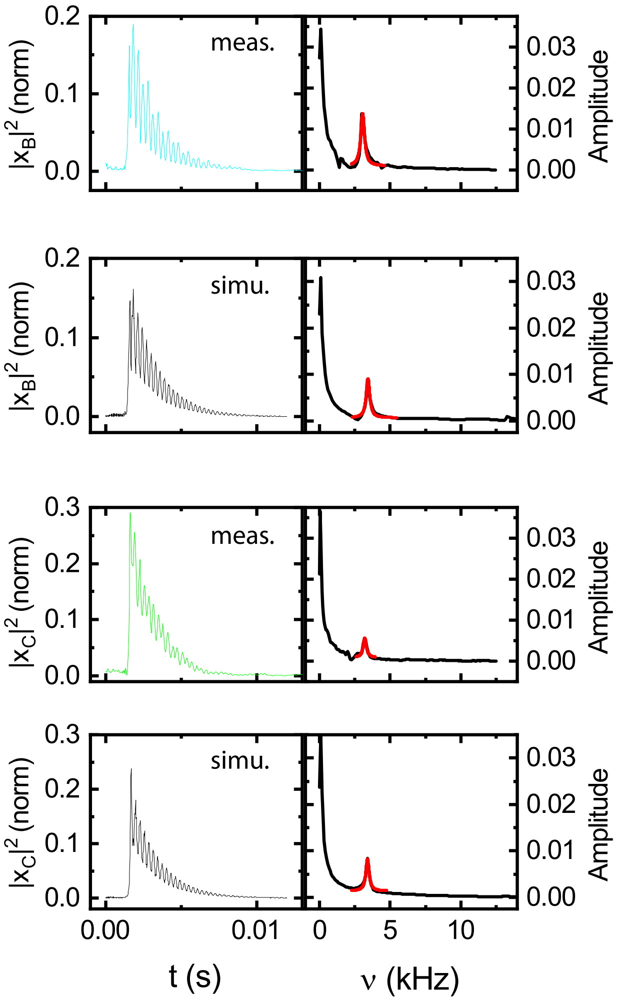


FIG. S2. Method used to extract the beating frequency in Fig. 4 b-f) in the main tesxt. Single slices at $(\zeta_\alpha/2\pi)^{-1} = 25\,\mu\mathrm{s/kHz}$ are shown for both resonators (B/C) from the experimental data as well as numerical simulation in the left column. The right column shows the Fourier transformation of the neighbouring data, the red line is a Lorentzian fit to the data, to extract the fast beating frequencies.

in Fig. 4. Here, we excite string A first with a short ($t_\mathrm{p}$) pulse with a sinusoidal force with the frequency $\Omega_\alpha$. Since $t_\mathrm{p} < t_0$ this can be written as $F_\mathrm{drive}(t) = F_0 \exp[i\Omega_\alpha^0 t]\Theta(t_\mathrm{p} - t)$ with the Heaviside step funciton $\Theta(t)$. We then use the ansatz $x_m(t) = x_0 c_m(t) \exp[i\Omega_\alpha(t)t]$ to find solutions for the amplitude coefficients $c_i(t)$ for all strings ($i$=A,B,C), with $|c_\mathrm{A}|^2 + |c_\mathrm{B}|^2 + |c_\mathrm{C}|^2 = 1$ . We now define the non hybridized frequencies of the remaining two strings B and C, using a generalized spring constant $\kappa_{ij}$ as $\Omega_{\beta,\gamma} = \sqrt{\kappa_{\beta\beta,\gamma\gamma}/m}$. Since $|\Omega_\alpha(t) - \Omega_{\beta,\gamma}| \ll \Omega_{\beta,\gamma}$ hold generally and $\Omega_\alpha(t) \approx \Omega_{\beta,\gamma}$ is true at the corresponding avoided crossings, we can use the time dependent frequency of mode $\alpha$ $\Omega_\alpha(t)$ to solve all three equations of motion (for modes $\alpha, \beta$ and $\gamma$) and obtain:

$$\ddot{c}_i G(t)\dot{c}_i + (F(t) + \Omega_i(t)c_i) = \frac{\kappa_{ij}}{m}c_j + \frac{\kappa_{ik}}{m}c_k + \frac{F_0}{mx_0}\Theta(t_\mathrm{p} - t) \tag{S9}$$

and with $F(t) = (i\dot{\Omega}_\alpha t + i\Omega_\alpha)^2 + 2i\dot{\Omega}_\alpha + \Gamma(i\dot{\Omega}_\alpha t + i\Omega_\alpha)$ and $G(t) = 2i(i\dot{\Omega}_\alpha t + \Omega_\alpha) + \Gamma$. Please note, that the spring constants mediating the coupling are much smaller compared to the effective spring constants of the resonators ($\kappa_{ij} \ll k_{ii}, i \neq j$). Therefore, we assume the amplitude coefficients $c_i(t)$ to vary much slower than the oscillatory motion of the strings. Due to this, we can neglect the second derivatives $\ddot{c}_i(t)$ and find the final form of the equations as:

$$G(t)\dot{c}_i + (F(t) + \Omega_\mathrm{A}^2(t))c_i = \frac{\kappa_{ij}}{m}c_j + \frac{\kappa_{ik}}{m}c_k + \frac{F_0}{mx_0}\Theta(t_\mathrm{p} - t) \tag{S10}$$

The numerical calculations have been carried out with *Wolfram Mathematica*.


[S1] S. Brundobler and V. Elser, Journal of Physics A: Mathematical and General **26**, 1211 (1993).
[S2] L. D. Landau, Z. Sowjetunion **2**, 46 (1932).
[S3] C. Zener, Proceedings of the Royal Society of London A **2**, 46 (1932).
[S4] G. H. Wannier, Physics Physique Fizika **1**, 251 (1965).
[S5] L. Novotny, American Journal of Physics **78**, 1199 (2010).
[S6] M. Pernpeintner, P. Schmidt, D. Schwienbacher, R. Gross, and H. Huebl, Physical Review Applied **10**, 034007 (2018).
[S7] A. Nayfeh, Nonlinear oscillations (Wiley, New York, 1979).
[S8] S. Timoshenko, W. Weaver, and D. Young, Vibration Problems in Engineering (John Wiley and Sons: New York, 1990 5th ed.).
